# Supplementary material for: Mind the Gap: Examining the Self-Improvement Capabilities of Large Language Models
Source: arXiv:2412.02674 source file (2025-02-25)
Supplement: Supplementary file 1 [file appendix_add_results.tex]

\begin{table}
    \centering
    \caption{}
    \resizebox{\linewidth}{!}{
    \begin{tabular}{c|c|c|cccc|ccc|c}
      \toprule
       \multirow{2}{*}{Name} & \multirow{2}{*}{Size} & \multirow{2}{*}{Accuracy} & \multicolumn{4}{c|}{MC} & \multicolumn{3}{c|}{CoT} & \multirow{2}{*}{To} \\ &&& top 0.7 & top 0.8 & $\tau = 0.7$ & $\tau = 0.8$ & Bin & S ($\tau = 8$) & S ($\tau = 9$) &  \\
    \midrule
    \multirow{7}{*}{Qwen 1.5} 
    & 0.5B & 0.1131 &-0.0914 &-0.1275 &-0.2901 &-0.2403 &-0.0002 &-0.0001 &0.0012 \\
    & 1.8B & 0.328 & 0.0743  &0.0752  &-0.003  &-0.0008 &0.0158  &0.0095  &0.0102 \\
    & 4B   & 0.502 & 0.0126  &0.0107  &0.0037  &0.0076  &0.0236  &0.0214  &0.0227 \\
    & 7B   & 0.531 & 0.0718  &0.0742  &0.0368  &0.0613  &0.0407  &0.0184 	&0.007  \\
    & 14B  & 0.638 & -0.0249 &-0.0411 &0.0233	 &0.0162  &0.0179  &0.0169  &0.02   \\
    & 32B  & 0.702 & -0.012  &-0.0258	&0.029   &0.0332  &0.0307  &0.0184	&0.019	\\
    & 72B  & 0.745 & 0.026   &0.0716	&0.0222	 &0.0294  &0.0355  &0.0247	&0.0291	\\
    \midrule 
    \multirow{4}{*}{Qwen 2} 
    & 0.5B &0.2619&0.0459	&0.0339	&0.0381	&-0.0659	&0.0021	&0.0064	&0.0072 &
    \\ 
    &1.5B &0.4882	&0.0609	&0.0527	&0.0502	&0.0132	&0.0126	&0.0278	&0.028\\ 
    &7B &0.7642	&0.0469	&0.0466	&0.039	&0.0217	&0.0236	&0.0197	&0.0208
    \\ 
    &72B &0.8169	&0.0239	&0.0238	&0.0089	&0.0212	&0.0251	&0.0208	&0.0245\\
    \midrule 
    \multirow{3}{*}{Llama 2}
    & 7B & 0.1164	&0.0233	&0.022	&0.001	&0	&0.0016	&0.0025	&0.0023 \\
    & 13B & 0.2157	&0.0345	&0.0318	&-0.0013	&0.0001	&0.0113	&0.0097	&0.0101\\
    & 70B & 0.4842	&0.0514	&0.0491	&0.0477	&0.0416	&0.0398	&0.0344	&0.0345\\
    \midrule 
    \multirow{2}{*}{Llama 3}
    & 8B & 0.4446	&0.0534	&0.0533	&-0.005	&0.0044	&0.0267	&0.021	&0.0213 \\
    & 70B & 0.7201	&0.0506	&0.0452	&0.0468	&0.0135	&0.0389	&0.0259	&0.0272\\
    \midrule 
    \multirow{2}{*}{Llama 3.1}
    & 8B & 0.4787	&0.0468	&0.0457	&-0.0225	&-0.0024	&0.0337	&0.0209	&0.0205 \\
    & 70B & 0.6988	&0.0688	&0.0677	&0.06	&0.0093&?	&0.0271	&0.0288\\
    \midrule
    \multirow{3}{*}{Yi 1.5}
    & 6B & 0.5553	&0.044	&0.0427	&0.0298	&-0.0097	&0.0201	&0.0188	&0.0195 \\
    & 9B & 0.6104	&0.0774	&0.075	&0.0561	&0.0573	&0.0232	&0.0361	&0.0372\\
    & 34B & 0.7371	&0.0629	&0.0623	&0.0334	&0.0484	&0.0249	&0.0286	&0.0295\\
    \bottomrule
    \end{tabular}\label{table:results}
    }
  \end{table}

  \begin{table}
    \centering
    \caption{}
    \resizebox{\linewidth}{!}{
    \begin{tabular}{c|c|c|cccc|ccc|c}
      \toprule
       \multirow{2}{*}{Name} & \multirow{2}{*}{Size} & \multirow{2}{*}{Accuracy} & \multicolumn{4}{c|}{MC} & \multicolumn{3}{c|}{CoT} & \multirow{2}{*}{To} \\ &&& top 0.7 & top 0.8 & $\tau = 0.7$ & $\tau = 0.8$ & Bin & S ($\tau = 8$) & S ($\tau = 9$) &  \\
      \midrule
      \multirow{7}{*}{Qwen 1.5} 
      & 0.5B & 0.1131 &-0.1951 &-0.2722 &-0.6196	&-0.5133&-0.0003	&-0.0013&0.0004 \\
      & 1.8B & 0.328 & 0.1588&0.1606 &-0.007 &-0.0018&0.0445	&0.031&0.0315 \\
      & 4B   & 0.502 & 0.0269&0.0228 &0.008	&0.0162	&0.0822&0.0692&0.0812 \\
      & 7B   & 0.531 & 0.1534&0.1584&0.0787	&0.1308	&0.1406	&0.055	&-0.0035 \\
      & 14B  & 0.638 & -0.0531 &-0.0879	&0.0497 &0.0346 	&0.0777	&0.08	&0.0902 \\
      & 32B  & 0.702 & -0.0257	&-0.055	&0.062	&0.0709	&0.1531	&0.084	&0.0849 \\
      & 72B  & 0.745 & 0.0555	&0.1528	&0.0474	&0.0629	&0.2182	&0.1496	&0.1697 \\
      \midrule 
      \multirow{4}{*}{Qwen 2} 
    & 0.5B &0.2619&0.0622	&0.0459	&0.0516	&-0.0893	&0.0044	&0.0158	&0.0179 &
      \\ 
    &1.5B &0.4882	&0.119	&0.103	&0.0982	&0.0258	&0.0445	&0.0996	&0.1011\\ 
    &7B &0.7642	&0.1989	&0.1974	&0.1653	&0.0918	&0.1646	&0.1373	&0.1434
    \\ 
    &72B &0.8169	&0.1307	&0.13	&0.0487	&0.1157	&0.2016	&0.1434	&0.1992\\
    \midrule 
    \multirow{3}{*}{Llama 2}
    & 7B & 0.1164	&0.0264	&0.0249	&0.0011	&0	&0.0025	&0.0039	&0.0037 \\
    & 13B & 0.2157& 0.044	&0.0405	&-0.0016	&0.0002	&0.0245	&0.0179	&0.0182\\
    & 70B & 0.4842& 0.0997	&0.0952	&0.0925	&0.0807	&0.1377	&0.1222	&0.1207\\
    \midrule 
    \multirow{3}{*}{Llama 2}
    & 7B & 0.1164	&0.0233	&0.022	&0.001	&0	&0.0016	&0.0025	&0.0023 \\
    & 13B & 0.2157	&0.0345	&0.0318	&-0.0013	&0.0001	&0.0113	&0.0097	&0.0101\\
    & 70B & 0.4842	&0.0514	&0.0491	&0.0477	&0.0416	&0.0398	&0.0344	&0.0345\\
    \midrule 
    \multirow{2}{*}{Llama 3}
    & 8B & 0.4446	&0.0962	&0.096	&-0.009	&0.008	&0.0851	&0.0616	&0.067 \\
    & 70B & 0.7201  &0.1808	&0.1613	&0.1671	&0.0484	&0.1909	&0.1324	&0.1374\\
    \midrule 
    \multirow{2}{*}{Llama 3.1}
    & 8B & 0.4787	&0.0897	&0.0877	&-0.0431	&-0.0047	&0.1174	&0.0702	&0.0689 \\
    & 70B & 0.6988	&0.2283	&0.2247	&0.1991	&0.0309	&0	&0.1265	&0.1359\\
    \midrule
    \multirow{3}{*}{Yi 1.5}
    & 6B & 0.5553	&0.0989	&0.096	&0.067	&-0.0217	&0.091	&0.066	&0.0669 \\
    & 9B & 0.6104	&0.1986	&0.1925	&0.144	&0.147	&0.1009	&0.1429	&0.1435\\
    & 34B & 0.7371	&0.2394	&0.2368	&0.127	&0.184	&0.1502	&0.1669	&0.1696\\
    \bottomrule
    \end{tabular}\label{table:results_relative}
    }
  \end{table}

\begin{table}
\centering
\caption{}
\resizebox{\linewidth}{!}{
\begin{tabular}{c|c|c|cccc|ccc|c}
    \toprule
    \multirow{2}{*}{Name} & \multirow{2}{*}{Size} & \multirow{2}{*}{Accuracy} & \multicolumn{4}{c|}{MC} & \multicolumn{3}{c|}{CoT} & \multirow{2}{*}{To} \\ &&& top 0.7 & top 0.8 & $\tau = 0.7$ & $\tau = 0.8$ & Bin & S ($\tau = 8$) & S ($\tau = 9$) &  \\
\midrule
\multirow{7}{*}{Qwen 1.5} 
& 0.5B & 11.31 &	-9.14 &	-12.75 &	-29.01 &	-24.03 &	-0.02 &	-0.01 &	0.12 & \\
& 1.8B & 32.81 &	7.43 &	7.52 &	-0.33 &	-0.08 &	1.58 &	0.95 &	1.02 & \\
& 4B   & 50.21 &	1.26 &	1.07 &	0.37 &	0.76 &	2.36 &	2.14 &	2.27 & \\
& 7B   & 53.17 &	7.18 &	7.42 &	3.68 &	6.13 &	4.07 &	1.84 &	0.70 &  \\
& 14B  & 63.87 &	-2.49 &	-4.11 &	2.33 &	1.62 &	1.79 &	1.69 &	2.00 &   \\
& 32B  & 70.25 &	-1.20 &	-2.58 &	2.90 &	3.32 &	3.07 &	1.84 &	1.90 &	\\
& 72B  & 74.55 &	2.60 &	7.16 &	2.22 &	2.94 &	3.55 &	2.47 &	2.91 &	\\
\midrule 
\multirow{4}{*}{Qwen 2} 
& 0.5B & 26.19 &	4.59 &	3.39 &	3.81 &	-6.59 &	0.21 &	0.64 &	0.72 &
\\ 
&1.5B & 48.82 &	6.09 &	5.27 &	5.02 &	1.32 &	1.26 &	2.78 &	2.80 &\\ 
&7B & 76.42 &	4.69 &	4.66 &	3.90 &	2.17 &	2.36 &	1.97 &	2.08 &
\\ 
&72B & 81.69 &	2.39 &	2.38 &	0.89 &	2.12 &	2.51 &	2.08 &	2.45 &\\
\midrule 
\multirow{3}{*}{Llama 2}
& 7B & 11.64 &	2.33 &	2.20 &	0.10 &	0.00 &	0.16 &	0.25 &	0.23 & \\
& 13B & 21.57 &	3.45 &	3.18 &	-0.13 &	0.01 &	1.13 &	0.97 &	1.01 &\\
& 70B & 48.42 &	5.14 &	4.91 &	4.77 &	4.16 &	3.98 &	3.44 &	3.45 &\\
\midrule 
\multirow{2}{*}{Llama 3}
& 8B & 44.46 &	5.34 &	5.33 &	-0.50 &	0.44 &	2.67 &	2.10 &	2.13 & \\
& 70B & 72.01 &	5.06 &	4.52 &	4.68 &	1.35 &	3.89 &	2.59 &	2.72 &\\
\midrule 
\multirow{2}{*}{Llama 3.1}
& 8B & 47.87 &	4.68 &	4.57 &	-2.25 &	-0.24 &	3.37 &	2.09 &	2.05 & \\
& 70B & 69.88 &	6.88 &	6.77 &	6.00 &	0.93 &	&2.71 &	2.88 &\\
\midrule
\multirow{3}{*}{Yi 1.5}
& 6B & 55.53 &	4.40 &	4.27 &	2.98 &	-0.97 &	2.01 &	1.88 &	1.95 & \\
& 9B & 61.04 &	7.74 &	7.50 &	5.61 &	5.73 &	2.32 &	3.61 &	3.72 &\\
& 34B & 73.71 &	6.29 &	6.23 &	3.34 &	4.84 &	2.49 &	2.86 &	2.95 &\\
\bottomrule
\end{tabular}\label{table:results_p}
}
\end{table}

\begin{table}
\centering
\caption{}
\resizebox{\linewidth}{!}{
\begin{tabular}{c|c|c|cccc|ccc|c}
    \toprule
    \multirow{2}{*}{Name} & \multirow{2}{*}{Size} & \multirow{2}{*}{Accuracy} & \multicolumn{4}{c|}{MC} & \multicolumn{3}{c|}{CoT} & \multirow{2}{*}{To} \\ &&& top 0.7 & top 0.8 & $\tau = 0.7$ & $\tau = 0.8$ & Bin & S ($\tau = 8$) & S ($\tau = 9$) &  \\
\midrule
\multirow{7}{*}{Qwen 1.5} 
& 0.5B & 11.31 &	-19.51 &	-27.22 &	-61.96 &	-51.33 &	-0.03 &	-0.13 &	0.04 &\\
& 1.8B & 32.81 &	15.88 &	16.06 &	-0.70 &	-0.18 &	4.45 &	3.10 &	3.15 & \\
& 4B   & 50.21 &	2.69 &	2.28 &	0.80 &	1.62 &	8.22 &	6.92 &	8.12 & \\
& 7B   & 53.17 &	15.34 &	15.84 &	7.87 &	13.08 &	14.06 &	5.50 &	-0.35 & \\
& 14B  & 63.87 &	-5.31 &	-8.79 &	4.97 &	3.46 &	7.77 &	8.00 &	9.02 &  \\
& 32B  & 70.25 &	-2.57 &	-5.50 &	6.20 &	7.09 &	15.31 &	8.40 &	8.49 &	\\
& 72B  & 74.55 &	5.55 &	15.28 &	4.74 &	6.29 &	21.82 &	14.96 &	16.97 &	\\
\midrule 
\multirow{4}{*}{Qwen 2} 
& 0.5B & 26.19 &	6.22 &	4.59 &	5.16 &	-8.93 &	0.44 &	1.58 &	1.79 &\\ 
&1.5B & 48.82 &	11.90 &	10.30 &	9.82 &	2.58 &	4.45 &	9.96 &	10.11 &\\ 
&7B & 76.42 &	19.89 &	19.74 &	16.53 &	9.18 &	16.46 &	13.73 &	14.34 &\\ 
&72B & 81.69 &	13.07 &	13.00 &	4.87 &	11.57 &	20.16 &	14.34 &	19.92 &\\
\midrule 
\multirow{3}{*}{Llama 2}
& 7B & 11.64 &	2.64 &	2.49 &	0.11 &	0.00 &	0.25 &	0.39 &	0.37 & \\
& 13B & 21.57 &	4.40 &	4.05 &	-0.16 &	0.02 &	2.45 &	1.79 &	1.82 &\\
& 70B & 48.42 &	9.97 &	9.52 &	9.25 &	8.07 &	13.77 &	12.22 &	12.07 &\\
\midrule 
\multirow{2}{*}{Llama 3}
& 8B & 44.46 &	9.62 &	9.60 &	-0.90 &	0.80 &	8.51 &	6.16 &	6.70 & \\
& 70B & 72.01 &	18.08 &	16.13 &	16.71 &	4.84 &	19.09 &	13.24 &	13.74 &\\
\midrule 
\multirow{2}{*}{Llama 3.1}
& 8B & 47.87 &	8.97 &	8.77 &	-4.31 &	-0.47 &	11.74 &	7.02 &	6.89 & \\
& 70B & 69.88 &	22.83 &	22.47 &	19.91 &	3.09 &	&	12.65 &	13.59 &\\
\midrule
\multirow{3}{*}{Yi 1.5}
& 6B & 55.53 &	9.89 &	9.60 &	6.70 &	-2.17 &	9.10 &	6.60 &	6.69 & \\
& 9B & 61.04 &	19.86 &	19.25 &	14.40 &	14.70 &	10.09 &	14.29 &	14.35 &\\
& 34B & 73.71 &	23.94 &	23.68 &	12.70 &	18.40 &	15.02 &	16.69 &	16.96 &\\
\bottomrule
\end{tabular}\label{table:relative_p}
}
\end{table}
